# Supplementary material for: Quantitative evaluation of defect-models in superconducting phase qubits
Source: arXiv:1010.6037 source file (2010-10-28)
Supplement: Supplementary file 1 [file lclimits_supp.pdf]

# Supplementary material to "Quantitative evaluation of defect models in superconducting phase qubits"


J. H. Cole,[1,2] C. Müller,[3,2] P. Bushev,[4,2] G. J. Grabovskij,[4]
J. Lisenfeld,[4] A. Lukashenko,[4] A. V. Ustinov,[4,2] and A. Shnirman[3,2]

[1] *Institut für Theoretische Festkörperphysik, Karlsruhe Institute of Technology, D-76128 Karlsruhe, Germany*
[2] *DFG-Center for Functional Nanostructures (CFN), D-76128 Karlsruhe, Germany*
[3] *Institut für Theorie der Kondensierten Materie, Karlsruhe Institute of Technology, D-76128 Karlsruhe, Germany*
[4] *Physikalisches Institut, Karlsruhe Institute of Technology, D-76128 Karlsruhe, Germany*


(Dated: October 28, 2010)


## Results of the fitting

The fitting was performed for an interaction Hamiltonian of the form

$$H_I = \hat{o}\left(\tilde{v}_\perp \tau_x + \tilde{v}_\parallel \tau_z\right) , \tag{S-1}$$

where the qubit operator $\hat{o}$ is given by the actual operator of the interaction and the $\tilde{v}$ are free parameters. In terms of the equations (3)-(5) the fitting parameters $\tilde{v}$ can be identified as

$$\tilde{v}_\perp = v_o \cos\theta_o \qquad \tilde{v}_\parallel = v_o \sin\theta_o . \tag{S-2}$$

Our experiment is only sensitive to purely transversal $\propto \sigma_x\tau_x$ and purely longitudinal $\propto \sigma_z\tau_z$ coupling. Mixed terms (e.g. $\propto \sigma_z\tau_x$ or $\propto \sigma_x\tau_z$) are not visible in the spectrum. If we were to ignore the higher lying qubit states, in the two state basis for the qubit we can write the relevant coupling Hamiltonian as

$$H_I = v_\perp \sigma_x\tau_x + v_\parallel \sigma_z\tau_z . \tag{S-3}$$

We then use the fitted values of $\tilde{v}$ to obtain the transversal and longitudinal coupling strengths

$$\begin{aligned} v_\perp &= \langle\hat{o}\rangle_\perp \tilde{v}_\perp , \\ v_\parallel &= \langle\hat{o}\rangle_\parallel \tilde{v}_\parallel , \end{aligned}$$

where the factors $\langle\hat{o}\rangle$ are given by

$$\begin{aligned} 2\langle\hat{o}\rangle_\perp &= \langle 1|\hat{o}|0\rangle + \langle 0|\hat{o}|1\rangle , \\ 2\langle\hat{o}\rangle_\parallel &= \langle 1|\hat{o}|1\rangle - \langle 0|\hat{o}|0\rangle . \end{aligned}$$

The table I gives the fitting results for two TLSs that were found on the same chip during one cooldown. Since the dataset for the second is smaller, the resulting uncertainties are bigger.

Since the momentum operator $\hat{q}$ has no diagonal components, $\langle\hat{q}\rangle_\parallel = 0$, no purely longitudinal coupling term exists in this case and we have no information on $\tilde{v}_\parallel$.

## Coupling to charge

Analogous to the treatment in Ref. [1] we calculate the fractional size $d$ of the aligned dipole moment in the direction of the electric field as

| TLS1 | $\epsilon_{\rm TLS}$ | $v_\perp$ | $v_\parallel$ | $\chi^2_r$ |
|---|---|---|---|---|
| $H_I^{(p)}$ | $7944.49 \pm 0.08$ | $35.65 \pm 0.08$ | $----$ | 0.998 |
| $H_I^{(\phi)}$ | $7944.41 \pm 0.08$ | $35.55 \pm 0.09$ | $0.23 \pm 0.12$ | 0.997 |
| $H_I^{(c)}$ | $7944.38 \pm 0.08$ | $35.52 \pm 0.13$ | $0.27 \pm 0.12$ | 0.997 |
| TLS2 | $\epsilon_{\rm TLS}$ | $v_\perp$ | $v_\parallel$ | $\chi^2_r$ |
| $H_I^{(p)}$ | $7734.0 \pm 0.2$ | $23.2 \pm 0.2$ | $----$ | 0.994 |
| $H_I^{(\phi)}$ | $7734.5 \pm 0.2$ | $23.3 \pm 0.2$ | $0.5 \pm 0.2$ | 0.992 |
| $H_I^{(c)}$ | $7734.4 \pm 0.3$ | $23.3 \pm 0.2$ | $0.5 \pm 0.2$ | 0.992 |

TABLE I: Estimates for the TLS resonance frequency and qubit-TLS coupling which were obtained from the fitting procedure, including 1-$\sigma$ uncertainties. The parameters for two different TLSs on the same chip are shown and all values are in MHz. The reduced $\chi^2$ value is also given for each fit, showing good convergence with minimal over-fitting.

$$d/x = v_\perp \sqrt{\frac{2C}{e^2\epsilon_{01}}} , \tag{S-4}$$

where $x$ ist the thickness of the junction, $C$ its capacitance and $e$ the electron charge. The qubit level splitting $\epsilon_{01}$ is taken in resonance with the TLS ($\epsilon_{01} = \epsilon_{\rm TLS}$) and $v_\perp$ is the transversal coupling strength from the fitting.

For the two TLSs under consideration we obtain

$$\begin{aligned} d_1/x &= 0.0837 \pm 0.0002 , \\ d_2/x &= 0.0551 \pm 0.0004 , \end{aligned}$$

where the subscript $1,2$ denotes TLS 1 / TLS 2 respectively.

For a junction thickness $x$ of $\propto$ nm, this results in an aligned dipole-size of the order of atomic distances.

## Coupling to external flux

We express the coupling operator in the Hamiltonian in the qubits 2-state representation as

$$\frac{\partial H}{\partial\phi_{Ext}}\delta\phi_{Ext} = \delta\phi_{Ext}\left(\eta_x\sigma_x + \eta_z\sigma_z\right) , \tag{S-5}$$

which we calculate using the full numeric qubit potential. For the numerical values of the parameters we obtain

$$\begin{aligned}\eta_{z,1} &= 3.57 \pm 0.04\,\text{GHz}\,\hbar/2\text{e}\,,\\ \eta_{x,1} &= 24.36 \pm 0.05\,\text{GHz}\,\hbar/2\text{e}\,,\\ \eta_{z,2} &= 3.89 \pm 0.04\,\text{GHz}\,\hbar/2\text{e}\,,\\ \eta_{x,2} &= 24.69 \pm 0.04\,\text{GHz}\,\hbar/2\text{e}\,.\end{aligned}$$

Comparing this with the results from the fitting to the operator $H_I^\phi = v_\phi \hat{\phi}\,(\cos\theta_\phi \tau_x + \sin\theta_\phi \tau_z)$ we can identify

$$\begin{aligned}v_\perp &= \delta\phi_{Ext}\eta_x \cos\theta_\phi\,,\\ v_\parallel &= \delta\phi_{Ext}\eta_z \sin\theta_\phi\,,\end{aligned}$$

with the definitions of $v_\perp$ and $v_\parallel$ given above. We solve this set of equations to get estimates for the change in magnetic flux $\delta\phi_{Ext}$ and the TLS orientation angle $\theta_\phi$:

$$\begin{aligned}\delta\phi_{Ext,1} &= 232.5 \pm 1.2\mu\Phi_0\,,\\ \delta\phi_{Ext,2} &= 151.5 \pm 2.5\mu\Phi_0\,,\end{aligned}$$

and

$$\begin{aligned}\tan\theta_{\phi,1} &= 0.04 \pm 0.02\,,\\ \tan\theta_{\phi,2} &= 0.14 \pm 0.06\end{aligned}$$

To estimate the magnetic moment needed to generate this change in external flux, we assume the moment to be located on the surface of the current carrying wire. The magnetic field on the surface of a wire of radius $R$ is given by

$$B = \frac{\mu_0}{2\pi}\frac{I}{R}\,, \tag{S-6}$$

with the direction parallel to the wire surface. The energy of a magnetic moment $\mu$ in a magnetic field is

$$U = -\vec{\mu}\cdot\vec{B}\,, \tag{S-7}$$

so the energy difference for the two possible orientations (parallel and anti-parallel) is given by

$$\delta E = 2\mu B\,. \tag{S-8}$$

A switching magnetic moment $\mu$ will induce a change in magnetic flux $\delta\Phi$ through a nearby ring. In order to calculate this change, we make use of Newton's third law, that a change $\delta\Phi$ in the magnetic flux through the loop induces an electromotive force due to Lenz' rule, which in turn gives an energy change of

$$\delta E = I\delta\Phi\,. \tag{S-9}$$

We compare the two energies and find the magnitude of the magnetic moment needed for a change in magnetic flux $\delta\Phi$ as

$$\mu = \frac{\pi R}{\mu_0}\delta\Phi\,, \tag{S-10}$$

which for our fits and a wire radius of $\propto 1\mu m$ gives us

$$\begin{aligned}\mu_1 &= 129700 \pm \phantom{0}700\,\mu_B\,,\\ \mu_2 &= \phantom{0}84500 \pm 1400\,\mu_B\,,\end{aligned}$$

in units of the electron magnetic moment $\mu_B$.

### Coupling to critical current

As in the case of the coupling to the external flux, we express the coupling operator in the Hamiltonian in the qubits 2-state representation as

$$\frac{\partial H}{\partial I_c}\delta I_c = \delta I_c\,(\lambda_x\sigma_x + \lambda_z\sigma_z)\,. \tag{S-11}$$

For the numerical values of the parameters we get

$$\begin{aligned}\lambda_{z,1} &= 8.91 \pm 0.07\,\text{GHz}/\mu\text{A}\\ \lambda_{x,1} &= 51.32 \pm 0.16\,\text{GHz}/\mu\text{A}\\ \lambda_{z,2} &= 9.45 \pm 0.07\,\text{GHz}/\mu\text{A}\\ \lambda_{x,2} &= 52.45 \pm 0.13\,\text{GHz}/\mu\text{A}\end{aligned}$$

Again comparing this with the results from the fitting to the operator $H_I^c = v_c \cos\hat{\phi}\,(\cos\theta_c\tau_x + \sin\theta_c\tau_z)$ we can identify

$$\begin{aligned}v_\perp &= \delta I_c\lambda_x\cos\theta_c\,,\\ v_\parallel &= \delta I_c\lambda_z\sin\theta_c\,,\end{aligned}$$

and obtain estimates for the change in critical current $\delta I_c$:

$$\begin{aligned}\delta I_{c,1} &= 693 \pm 5 \times 10^{-12}\text{A}\,,\\ \delta I_{c,2} &= 447 \pm 7 \times 10^{-12}\text{A}\,,\end{aligned}$$

where the critical current is obtained via our fitting procedure,

$$\begin{aligned}I_{c,1} &= 984 \pm 2 \times 10^{-9}\text{A}\,,\\ I_{c,2} &= 976 \pm 1 \times 10^{-9}\text{A}\,.\end{aligned}$$

The angle $\theta_c$ can be found as

$$\begin{aligned}\tan\theta_{c,1} &= 0.04 \pm 0.02\,,\\ \tan\theta_{c,2} &= 0.12 \pm 0.05\end{aligned}$$

Using these estimates for the angle $\theta$ we can place further constraints on the microscopic model. We can write the Hamiltonian in its physical basis, in which the coupling to the qubit is diagonal, (e.g., the position basis for a bistable atomic defect) as

$$H_{\text{TLS}} = \frac{1}{2}\epsilon_0\tilde{\tau}_z + \frac{1}{2}\Delta_0\tilde{\tau}_x\,, \tag{S-12}$$

where $\epsilon_0$ gives the splitting in the physical basis and $\Delta_0$ the tunneling element between the two states. The

coupling operator in the eigenbasis is then given by $\tilde{\tau}_z \to \cos\theta\,\tau_x + \sin\theta\,\tau_z$ with $\tan\theta = \epsilon_0/\Delta_0$, while the level splitting of the TLS is calculated as $\epsilon_{\rm TLS} = \sqrt{\epsilon_0^2 + \Delta_0^2}$. Therefore, an angle of $\theta = \pi/2$ would correspond to exact degeneracy of the TLS-states in the original basis. Using the above estimates yields

$$\begin{aligned} \epsilon_{0,1} &= 0.34 \pm 0.16\,\mathrm{GHz}\,, \\ \Delta_{0,1} &= 7.937 \pm 0.007\,\mathrm{GHz}\,, \\ \epsilon_{0,2} &= 0.97 \pm 0.38\,\mathrm{GHz}\,, \\ \Delta_{0,2} &= 7.89 \pm 0.05\,\mathrm{GHz}\,. \end{aligned}$$

## Andreev level fluctuator

Ref. 2 gives a general model for coupling between a qubit and an Andreev level fluctuator (ALF), formed when an impurity level in the Josephson junction is hybridised with the superconducting leads. The Hamiltonian for this model is given as

$$\begin{aligned} H = &\frac{1}{2}\epsilon_q\sigma_z + E_b\tau_z \\ &+ (v_z\sigma_z + v_x\sigma_x)\left(2\sqrt{a_+a_-}\tau_x + (a_+ - a_-)\tau_z\right) \end{aligned} \tag{S-13}$$

(Eq. (35) in ref. 2), where we slightly adapted their notation to our convention. The operators $\sigma$ and $\tau$ are the pauli-matrices for qubit and TLS, respectively. Comparing eq. (S-13) with eq. (S-3) we can identify

$$\begin{aligned} 2\sqrt{a_+a_-} &= \cos\theta \\ (a_+ - a_-) &= \sin\theta \end{aligned} \tag{S-14}$$

The amplitudes $a_\pm$ are given by

$$a_\pm = \frac{(\Delta_{\rm BCS}^2 - E_b^2)\left[(\epsilon_d \pm E_b)^2 + \gamma^2\right]}{2\left[(2\Delta_{\rm BCS}^2 - E_b^2)(\epsilon_d^2 + \gamma^2) - E_b^4\right]}\,, \tag{S-15}$$

while the Andreev level splitting $E_b$ is the solution to

$$E_b^2\left(1 + \frac{2\gamma}{\sqrt{\Delta_{\rm BCS}^2 - E_b^2}}\right) - \epsilon_d^2 - \gamma^2 = 0\,. \tag{S-16}$$

Here $\Delta_{\rm BCS}$ is the superconducting gap ($\Delta_{\rm BCS} \approx 300\mu$eV for thin Al-films), $\epsilon_d$ is the impuritiy level energy and $\gamma$ is the hybridisation parameter characterizing the interaction with the leads. The ALF splitting $E_b$ is related to the TLS energy splitting $\epsilon_{\rm TLS}$ in our model by $2E_b = \epsilon_{\rm TLS}$. Inserting eq. (S-16) into eq. (S-15) we can express the amplitudes $a_\pm$ as function of only one unknown variable, the impurity level energy $\epsilon_d$. The relations (S-14) therefore connect the angle $\theta$ in this model to the impurity level energy $\epsilon_d$.

In the model of Ref. 2 the coupling between qubit and ALF is via a modulation of the critical current $I_c$. The coupling paramteters $v_{x/z}$ in eq. (S-13) are then given by $v_{x/z} = \delta I_c\lambda_{x/z}$, with $\lambda_{x/z}$ defined by eq. (S-11).

Comparing now eq. (S-13) with our fitted results we find the system of coupled equations

$$\begin{aligned} v_\perp &= 2\lambda_x\delta I_c\sqrt{a_+a_-}\,, \\ v_\parallel &= \lambda_z\delta I_c(a_+ - a_-)\,, \end{aligned} \tag{S-17}$$

which we can solve for the two unknowns critical current variation $\delta I_c$ and the impurity level energy $\epsilon_d$. Solving these equations will give us a multitude of possible solutions, from which we will only show the largest values. Fig. 1 shows the full spectrum of solutions.

For the values of $v_\perp$ and $v_\parallel$ we obtain in the fitting we get a change in critical current of

$$\begin{aligned} \delta I_{c,1} &\leq 1.46 \pm 0.01 \times 10^{-9}\mathrm{A} \\ \delta I_{c,2} &\leq 0.94 \pm 0.01 \times 10^{-9}\mathrm{A} \end{aligned}$$

and an impurity level energy of

$$\begin{aligned} \epsilon_{d,1} &\leq 101.6 \pm 46.5\,\mathrm{MHz} \\ \epsilon_{d,2} &\leq 278.4 \pm 109.6\,\mathrm{MHz} \end{aligned}$$

To illustrate the dependence of these two variables on the longitudinal coupling $v_\parallel$, we plot their values as a function of $v_\parallel$ in a range of $[-5, 5]$ times the fitted value. The result is shown in Fig. 1.

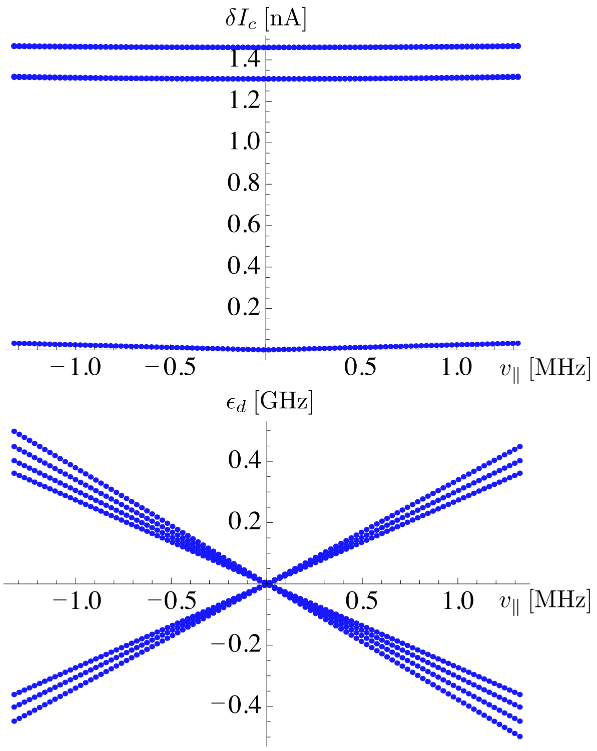


FIG. 1: Change in critical current $\delta I_c$ (upper plot) and impurity level energy $\epsilon_d$ (lower plot) as a function of longitudinal coupling $\tilde{v}_\parallel$ and for constant transversal coupling strength $\tilde{v}_\perp$. Numbers are taken from the fitted values for TLS 1. The range in longitudinal coupling is $\pm 5$ times the fitted result.

[1] J. M. Martinis, K. B. Cooper, R. Mcdermott, M. Steffen, M. Ansmann, K. D. Osborn, K. Cicak, S. Oh, D. P. Pappas, R. W. Simmonds, et al., Phys. Rev. Lett. **95** (2005).
[2] R. D. Sousa, K. B. Whaley, T. Hecht, J. V. Delft, and F. K. Wilhelm, Phys. Rev. B **80**, 094515 (2009).
